# Supplementary material for: Predicting Future Cognitive Decline with Hyperbolic Stochastic Coding
Source: arXiv:2102.10503 source file (2021-02-21)
Supplement: Supplementary file 1 [file Appendix.tex]

%\vspace{-4mm}
\newpage
\begin{center}
{\large Appendix}
\end{center}
\appendices
%\section{APPENDIX}

%\vspace{-4mm}
\section{Convergence Analysis of Stochastic Coordinate Coding}
\label{App:converge}
Here we show that our algorithm is convergent. The objective function ${\cal F}$ in Eq.~\ref{eq:opt} can be re-written as follows:
\small
\begin{equation}\label{eq:obj-scc-ca}
\mathcal{F}(\mathbf{D}, \mathbf{z}_1, \cdots, \mathbf{z}_n) = \frac{1}{n}\sum_{i=1}^n (\frac{1}{2}\| \mathbf{Dz}_i - \mathbf{x}_i \|^2_2 + \lambda \| \mathbf{z}_i \|_1).
\end{equation}
\normalsize
It is clear that ${\cal F}(\mathbf{D}, \mathbf{z}_1, \cdots, \mathbf{z}_n)$ is a nonnegative continuous function over a bounded set $\mathbf{D}\in \mathbb{C}$ and
$\|\mathbf{z}_i\|\le M$ for a real number $M<\infty$, ${\cal F}(\mathbf{D}, \mathbf{z}_1, \cdots, \mathbf{z}_n)\to \infty$ if $\|\mathbf{z}_i\|_1
\to \infty$. Thus, the minimization problem (Eq.~\ref{eq:obj-scc-ca}) has a solution. As the minimization functional ${\cal F}$ is not a convex function, the problem (Eq.~\ref{eq:obj-scc-ca}) may have multiple solutions and we show our algorithm convergence under certain conditions.

The proof is divided into three parts. We first show the convergence analysis for updating sparse codes (CD step) and updating dictionary (SGD step), respectively. We then combine these two parts to show the convergence of the stochastic coordinate coding (SCC).
%\vspace{-4mm}
\subsection{Convergence Analysis of the CD Step}
First, we analyze the convergence of CD step. Suppose we update the $j$-th coordinate $z^k_{i, j}$ of $\mathbf{z}^k_i$ in our cyclic selection approach. It is clear that
\small
\[
z^k_{i, j} = \arg\min_{\mathbf{z}} f_i(\mathbf{D}^k_i, z^{k}_{i, 1}, \cdots, z^{k}_{i, j-1}, z_{i, j}^k , z^{k-1}_{i, j+1}, \cdots, z^{k-1}_{i, t}).
\]
\normalsize
Therefore, after going through the whole cycle, we obtain the following result.
%\begin{Prop}\label{prop:cd--z-dec}
%For any $k$ and $i$, we have
%\end{Prop}
%\small
%\begin{equation}\label{eq:cd-z-dec}
%f_i (\mathbf{D}^k_{i}, \mathbf{z}_i^{k}) \leq f_i %(\mathbf{D}^k_{i}, \mathbf{z}_i ).
%\end{equation}
\normalsize
\begin{Prop}\label{prop:cd--z-dec}
\textbf{For any $k$ and $i$, we have}
%Let $L > \|\mathbf{D}_i^k \|^2$ be a positive number. %Then
\small
\begin{equation}\label{eq:cd-z-dec}
f_i (\mathbf{D}^k_{i}, \mathbf{z}_i^{k}) \leq f_i (\mathbf{D}^k_{i}, \mathbf{z}^{k-1}_i ).
\end{equation}
\normalsize
\textbf{Further, we have $f_i (\mathbf{D}^k_{i}, \mathbf{z}_i^{k}) \leq f_i (\mathbf{D}^k_{i}, \mathbf{z}_i^{k-1}) - \gamma\|\mathbf{z}_i^k- \mathbf{z}_i^{k-1}\|^2$ for a constant $\gamma>0$.}
\end{Prop}

\emph{Proof.}
\textbf{For simplicity, we let $f_i(\mathbf{D}^k_{i},\mathbf{z}^k_i) = \ell(\mathbf{D}^k_{i},\mathbf{z}^k_i) + \lambda \|\mathbf{z}_i^k \|_1$. Then we can use Taylor expansion of $\ell(\mathbf{D}^k_{i},\mathbf{z}^k_i)$ at $\mathbf{z}_i^{k-1}$ to rewrite $\ell(\mathbf{D}^k_{i}, \mathbf{z}_i^k) $ into}
\small
\begin{equation}
\begin{aligned}
\label{eq:CD1}
&\ell(\mathbf{D}^k_{i}, \mathbf{z}_i^k) = \ell(\mathbf{D}^k_i,\mathbf{z}_i^{k-1}) + \langle \nabla \ell(\mathbf{D}^k_{i},\mathbf{z}_i^{k-1}), \mathbf{z}_i^k-\mathbf{z}_i^{k-1}\rangle +  \frac{1}{2}\|\mathbf{D}_i^k (\mathbf{z}_i^k-\mathbf{z}_i^{k-1})\|^2 
\\ \leq & \ell(\mathbf{D}^k_i,\mathbf{z}_i^{k-1}) + \langle \nabla \ell(\mathbf{D}^k_{i},\mathbf{z}_i^{k-1}), \mathbf{z}_i^k-\mathbf{z}_i^{k-1}\rangle
+ \frac{\| \mathbf{D}_i^k\|^2 }{2}\|\mathbf{z}_i^k-\mathbf{z}_i^{k-1}\|^2
\end{aligned}
\end{equation}
\normalsize
\textbf{As shown in~\citep{lin2014stochastic}, $\mathbf{z}_i^k$ is a minimizer of Eq.~\ref{eq:cd-obj-a}. Therefore, we have the following equation:}
\small
\begin{equation}
\begin{aligned}
\label{eq:CD2}
&\mathrm{CD}( \mathbf{z}_i^{k}, \mathbf{D}^k_i, \mathbf{x}_i, \mathbf{z}_i^{k-1} ) 
= \langle \nabla \ell(\mathbf{D}^k_{i},\mathbf{z}_i^{k-1}), \mathbf{z}_i^k-\mathbf{z}_i^{k-1}\rangle + \frac{L}{2}\|\mathbf{z}_i^k- \mathbf{z}_i^{k-1}\|^2 + \lambda \| \mathbf{z}_i^k \|_1 \\
\leq &\mathrm{CD}( \mathbf{z}_i^{k-1}, \mathbf{D}^k_i, \mathbf{x}_i, \mathbf{z}_i^{k-1} ) 
= \lambda \| \mathbf{z}_i^{k-1}\|_1.
\end{aligned}
\end{equation}
\normalsize
\textbf{We then add Eq.~\ref{eq:CD1} and Eq.~\ref{eq:CD2} together, and simplify the inequality, we have}
\small
\begin{align*}
\ell(\mathbf{D}^k_{i},\mathbf{z}_i^k) + \lambda \| \mathbf{z}_i^k \|_1& \le \ell(\mathbf{D}^k_{i},\mathbf{z}_i^{k-1}) + \lambda \| \mathbf{z}_i^{k-1} \|_1 - \frac{L-\| \mathbf{D}_i^k \|^2}{2} \|\mathbf{z}_i^k- \mathbf{z}_i^{k-1}\|^2 \\
f(\mathbf{D}^k_{i},\mathbf{z}_i^{k}) &= f(\mathbf{D}^k_{i},\mathbf{z}_i^{k-1}) - \gamma \|\mathbf{z}_i^k- \mathbf{z}_i^{k-1}\|^2,
\end{align*}
\normalsize
\textbf{where $L > ||\mathbf{D}_i^k||^2$ is the Lipschitz constant, so $\gamma = (L-\| \mathbf{D}_i^k \|^2)/2 > 0$. }

If there are $q$ steps using CD, we should have
\small
\begin{equation}
\label{keystep1}
f_i (\mathbf{D}^k_{i}, \mathbf{z}_i^{k+q}) \leq f_i (\mathbf{D}^k_{i}, \mathbf{z}^{k-1}_i ).
\end{equation}%{$\square$}
\hfill{$\square$}
\normalsize

When $q$ is sufficiently large, we know that $f_i(\mathbf{D}_i^k,\mathbf{z}_i^{k+q})$ decreases to the minimum value $f_i^* = \min_{z} f_i(\mathbf{D}_i^k,\mathbf{z})$.
Since $f_i(\mathbf{D}_i^k, \mathbf{z})$ is a convex function,  $f^*_i \le f_i(\mathbf{D}_i^k,0) = \dfrac{1}{2}\|\mathbf{x}_i\|^2 =1/2$. It follows that $\|\mathbf{z}_i^{k+q}\|_1 \le \frac{1}{2\lambda}$. This analysis works for all $i=1, \cdots, n$ and for any $k, q$. We take enough steps so that $f_i(\mathbf{D}^k_i, \mathbf{z}_i^{k+q}) \le 1/2$. Therefore, we have the following results for the output $\mathbf{z}_i^k$:
\begin{Prop}
\label{bound}
If the number of iterative steps for the CD is sufficiently large, all $\mathbf{z}_i^k$ are uniformly bounded for $i=1, \cdots, n$ and $k\ge 1$.
\end{Prop}

It might be worth noting that in practice performing only a small number steps of CD is sufficient to guarantee that all $\mathbf{z}_i^k$ are uniformly bounded.

%\vspace{-1em}
\subsection{Convergence Analysis of the SGD Step}
Second, we study the SGD step. Note that we can always re-index $\mathbf{D}^k_i$ as $\mathbf{D}_{(k-1)n+i+1}$ for convenience. To simplify the notation, we omit the superscript $k$ on the dictionary $\mathbf{D}$ and the learning rate $\eta$ in this section.
Our SGD step in Eq.~\ref{eq:sgd} is equivalent to the following two sub-steps by using proximal gradient method~\citep{parikh2014proximal}.
\small
\begin{equation}\label{eq:sgd-step1}
\hat{\mathbf{D}}_{i+1} = \arg \min_\mathbf{D} g_i(\mathbf{D}_i) + \langle \nabla g_i(\mathbf{D}_i), \mathbf{D} - \mathbf{D}_i \rangle + \frac{1}{2\eta_i} \| \mathbf{D} - \mathbf{D}_i \|^2_2,
\end{equation}
\begin{equation}\label{eq:sgd-step2}
\mathbf{D}_{i+1} = P_{\mathbb{C}} (\hat{\mathbf{D}}_{i+1}) =  \arg\min_{\mathbf{D} \in \mathbb{C}} \| \hat{\mathbf{D}}_{i+1} - {\mathbf{D}} \|.
\end{equation}
\normalsize
For simplicity, we let $g_{i}(\mathbf{D}) \equiv \frac{1}{2} \| \mathbf{Dz}^k_i - \mathbf{x}_i \|^2_2 $. Next we show that $g_i$ decreases after performing SGD.
\begin{Prop}
$g_i(\hat{\mathbf{D}}_{i+1}) \leq g_i(\mathbf{D}_i)$ if $\eta_i \le \frac{1}{L}$.
\end{Prop}

\emph{Proof.}
We use Taylor expansion of $g_i$ at $\mathbf{D}_i$ and the Lipschitz differentiation of $g_i(\mathbf{D})$, we have
\small
\[
\begin{aligned}
g_i(\hat{\mathbf{D}}_{i+1}) &= g_i (\mathbf{D}_i) + \langle \nabla g_i (\mathbf{D}_i), \hat{\mathbf{D}}_{i+1} - \mathbf{D}_i \rangle + \frac{L}{2} \| \hat{\mathbf{D}}_{i+1} - \mathbf{D}_i \|^2 \\
&\leq g_i (\mathbf{D}_i) + \langle \nabla g_i (\mathbf{D}_i), \hat{\mathbf{D}}_{i+1} - \mathbf{D}_i \rangle + \frac{1}{2\eta_i} \| \hat{\mathbf{D}}_{i+1} - \mathbf{D}_i \|^2 \\
&\leq g_i (\mathbf{D}_i) + \langle \nabla g_i (\mathbf{D}_i), \mathbf{D}_i - \mathbf{D}_i \rangle + \frac{1}{2\eta_i} \| \mathbf{D}_i - \mathbf{D}_i \|^2 \\
&=g_i(\mathbf{D}_i),
\end{aligned}
\]
\normalsize
where the third inequality is due to the optimality condition of Eq.~\ref{eq:sgd-step1} and $L$ is Lipschitz constant.\hfill $\square$
%\rightline{$\square$}

\begin{Prop}\label{claim:sgd-dec}
$g_i({\mathbf{D}}_{i+1}) \leq g_i(\mathbf{D}_i)$ if $\eta_i \| \mathbf{z}^k_i \|^2\le 1$.
\end{Prop}
\emph{Proof.}
Note that $ \| \hat{\mathbf{D}}_{i+1} - \mathbf{D}_{i+1} \| \leq  \| \hat{\mathbf{D}}_{i+1} - \mathbf{D}_i \|$ by Eq.\ref{eq:sgd-step2}. By a direct computation of CD in Eq.\ref{eq:sgd-step1}, we have
$
\hat{\mathbf{D}}_{i+1}  = \mathbf{D}_i - \eta_i \nabla g_i(\mathbf{D}_i) 
$
because $\hat{\mathbf{D}}_{i+1}$ is the proximation of $\mathbf{D}_i - \eta_i \nabla g_i(\mathbf{D}_i) $.
Thus
\small
\[
\begin{aligned}
\label{eq:above}
 \| \hat{\mathbf{D}}_{i+1} - \mathbf{D}_{i+1} \|^2 = \|  \mathbf{D}_i - \eta_i \nabla g_i(\mathbf{D}_i) - \mathbf{D}_{i+1} \|^2 \leq  \| \hat{\mathbf{D}}_{i+1} - \mathbf{D}_i \|^2 = \| \eta_i \nabla g_i(\mathbf{D}_i) \|^2.
\end{aligned}
\]
\normalsize
Then, we expand the left side of the above inequality and have
\small
\begin{equation}\label{eq:inequ-norm-inner}
\| \mathbf{D}_{i+1} - \mathbf{D}_i \|^2  \leq -2 \eta_i  \langle \mathbf{D}_{i+1} - \mathbf{D}_i, \nabla g_i(\mathbf{D}_i)\rangle .
\end{equation}
\normalsize
According to the definition of $g_i$, we have
\small
\begin{eqnarray*}
 g_i(\mathbf{D}_{i+1}) &=& \frac{1}{2} \| \mathbf{D}_{i+1} \mathbf{z}_i^k - \mathbf{x}_i \|^2 \\
&=& \frac{1}{2} \| (\mathbf{D}_{i+1} - \mathbf{D}_i) \mathbf{z}_i^k + \mathbf{D}_i\mathbf{z}_i^k - \mathbf{x}_i \|^2 \\
&=& \frac{1}{2} \| \mathbf{D}_{i+1} - \mathbf{D}_i\|^2 \| \mathbf{z}_i^k\|^2 + \langle  (\mathbf{D}_{i+1} - \mathbf{D}_i) \mathbf{z}_i^k,  \mathbf{D}_i\mathbf{z}_i^k - \mathbf{x}_i \rangle +  g_i(\mathbf{D}_i) \\
&\leq& -\eta_i \| \mathbf{z}_i^k\|^2 \langle \mathbf{D}_{i+1} - \mathbf{D}_i, \nabla g_i(\mathbf{D}_i)  \rangle + \langle  (\mathbf{D}_{i+1} - \mathbf{D}_i) \mathbf{z}_i^k,   \mathbf{D}_i\mathbf{z}_i^k - \mathbf{x}_i \rangle +  g_i(\mathbf{D}_i) \\
&=& -\eta_i  \| \mathbf{z}_i^k\|^2 \langle  \mathbf{D}_{i+1} - \mathbf{D}_i,  \nabla g_i(\mathbf{D}_i)   \rangle + \langle  \mathbf{D}_{i+1} - \mathbf{D}_i , \nabla g_i(\mathbf{D}_i)\rangle +  g_i(\mathbf{D}_i) \\
&=& (1 -\eta_i  \| \mathbf{z}_i^k\|^2) \langle \mathbf{D}_{i+1} - \mathbf{D}_i,  \nabla g_i(\mathbf{D}_i)   \rangle   +  g_i(\mathbf{D}_i)
\end{eqnarray*}
\normalsize
By Eq.~\ref{eq:inequ-norm-inner}, we get $ \langle  \mathbf{D}_{i+1} - \mathbf{D}_i, \nabla g_i(\mathbf{D}_i) \rangle \leq -\frac{1}{2\eta_i}
\| \mathbf{D}_{i+1} - \mathbf{D}_i \|^2 \leq 0$. If $\eta_i \leq \frac{1}{\| \mathbf{z}_i^k \|^2}$, we have $g_i(\mathbf{D}_{i+1}) \leq g_i(\mathbf{D}_i)$.
 \hfill $\square$

Since $\|\mathbf{z}_i^k\|_1, i\ge 1, k\ge 1$ are uniformly bounded as in Proposition~\ref{bound}, $g_i(\mathbf{D}_{i+1}) \le G$ for a positive constant $G$ independent of $i$. Furthermore, we have $\nabla g_i(\mathbf{D}_i^k) = (\mathbf{D}_i^k \mathbf{z}_i^k -\mathbf{x}_i)(\mathbf{z}_i^k)^T$ and it is easy to see that $\|\nabla g_i(\mathbf{D}_i^k)\|\le C^2$ for a positive constant $C$. Thus, we have
\begin{Prop}
Suppose $\|\nabla g_i(\mathbf{D}_i^k) \|^2 \leq C^2$ for all $i$ and $k$, then
$
\| \mathbf{D}_{i+1} -  \mathbf{D}_i \| \leq 2\eta_i C.
$
\end{Prop}
\emph{Proof.}
With Eq.~\ref{eq:inequ-norm-inner}, we have
\small
\begin{align*}
\| \mathbf{D}_{i+1} - \mathbf{D}_i \|^2  &\leq -2 \eta_i  \langle \nabla g_i(\mathbf{D}_i), \mathbf{D}_{i+1} - \mathbf{D}_i \rangle \\
&\leq 2\eta_i \|  \nabla g_i(\mathbf{D}_i)  \| \, \|\mathbf{D}_{i+1} - \mathbf{D}_i  \| \\
&\leq 2\eta_i C \|\mathbf{D}_{i+1} - \mathbf{D}_i  \|.
\end{align*}
\normalsize
The conclusion follows dividing both sides by $\|\mathbf{D}_{i+1} - \mathbf{D}_i\|$ if it is not zero. If it is zero, then the inequality in the proposition is obviously valid. \hfill $\square$

\iffalse
One can further prove that $\mathbf{D}_i$ is square summable, we then have the following
\begin{Coro}
\label{coro:di-d}
$$
\sum_{i=1}^\infty \| \mathbf{D}_i- \mathbf{D}_{i+1}\|^2 \le 4 C^2 \sum_{i=1}^\infty \frac{1}{(i+1)^2}<4C^2.
$$
\end{Coro}
\emph{Proof.}
Indeed, we have
\small
\begin{align*}
\| \mathbf{D}_{i+1} - \mathbf{D}_i \|^2  &\leq 2\eta_i \|  \nabla g_i(\mathbf{D}_i)  \| \, \|\mathbf{D}_{i+1} - \mathbf{D}_i  \| \\
&\le 2C^2  \eta_i^2 + \frac{1}{2}  \|\mathbf{D}_{i+1} - \mathbf{D}_i  \|^2
\end{align*}
\normalsize
by using Cauchy-Schwarz inequality.
$
\|\mathbf{D}_{i+1} - \mathbf{D}_i  \|^2 \le 4 C^2 \eta_i^2.
$
Summing over $i\ge 1$ concludes the desired inequality.\qquad\qquad\qquad\qquad\qquad\qquad\qquad\qquad\qquad\qquad\qquad\qquad\qquad\qquad\qquad{$\square$}
%\rightline{$\square$}
\fi

\subsection{Convergence Analysis of the HSC}
Now we can give the critical decreasing proposition.
\begin{Prop}\label{prop:exp-dic-dec}
For any epoch $k\ge 1$, we have
\small
\[
\frac{1}{n} \sum_{i=1}^n f_i(\mathbf{D}^k_{i+1}, \mathbf{z}_i^k) \leq \frac{1}{n} \sum_{i=1}^n f_i(\mathbf{D}^k_i, \mathbf{z}_i^{k-1}).
\]
\normalsize
\end{Prop}
\emph{Proof.}

With Proposition \ref{prop:cd--z-dec} we have
\small
\begin{equation}\label{eqn:fidizifidizik-1}
f_i(\mathbf{D}_{i}^k, \mathbf{z}_i^k) \leq f_i (\mathbf{D}_i^k, \mathbf{z}_i^{k-1}), 
\end{equation}

\normalsize
With Proposition~\ref{claim:sgd-dec}, we have
\small
\begin{equation}
g_i(\mathbf{D}_{i+1}^k, \mathbf{z}_i^k) + \lambda \| \mathbf{z}_i^k \|_1\leq g_i (\mathbf{D}_i^k, \mathbf{z}_i^k) +\lambda \| \mathbf{z}_i^{k} \|_1, 
\end{equation}

\normalsize
It is equivalent to
\small
\begin{equation}\label{eqn:gibyprop5}
f_i(\mathbf{D}_{i+1}^k, \mathbf{z}_i^k) \leq f_i (\mathbf{D}_i^k, \mathbf{z}_i^k). 
\end{equation}

\normalsize
Combining Eq.~\ref{eqn:fidizifidizik-1} and Eq.~\ref{eqn:gibyprop5} and summing from $i=1$ to $n$, we get the desired inequality. \\\hfill $\square$

\begin{Prop}
\label{prop:di-d*}
Suppose that $\mathbf{D}^*\in \mathbb{C}$ (recall $\mathbb{C}$ is the feasible set of $\mathbf{D}$ in Eq.~\ref{eq:sgd}) is a local minimizer such that the mean value ${\cal E}(\nabla g_i(\mathbf{D}^*))=0$ over random variables $(\mathbf{z}, \mathbf{x})$.
Suppose $ g_i(\mathbf{D})$ is strongly convex~\citep{boyd2004convex}, so there exist $\eta_i = \frac{1}{(i+1)\beta } (\beta > 0)$ for any $i$ and $k$. Then the mean of the difference $\|\mathbf{D}_i - \mathbf{D}^*\|$ is
\[
{\cal E}(\| \mathbf{D}_{i} -  \mathbf{D}^* \|) \leq  \frac{1}{i+1}(1+ \ln(i+1) \frac{G^2}{\beta^2}),
\]
where in Prop.~\ref{bound}, $g_i(\mathbf{D}_{i+1}) \le G$ for a positive constant $G$ independent of $i$.
\end{Prop}
\begin{proof}
Due to the non-expansive property of the projection $P_{\mathbb{C}}$, we have
\begin{align*}
\| \mathbf{D}_{i+1} - \mathbf{D}^* \|^2 &= \| P_{\mathbb{C}}(\mathbf{D}_i - \eta_i \nabla g_i(\mathbf{D}_i)) - P_{\mathbb{C}}(\mathbf{D}^*) \|^2 \\
&\leq \|\mathbf{D}_i - \eta_i \nabla g_i(\mathbf{D}_i) - \mathbf{D}^* \|^2 \\
&= \| \mathbf{D}_i - \mathbf{D}^* \|^2 + \eta_i^2  \| \nabla g_i(\mathbf{D}_i) \|^2   - 2\eta_i  \langle \nabla g_i(\mathbf{D}_i), \mathbf{D}_i - \mathbf{D}^* \rangle  \\
&\leq \| \mathbf{D}_i - \mathbf{D}^* \|^2 + \eta_i^2 C^2 - 2\eta_i  \langle \nabla g_i(\mathbf{D}_i), \mathbf{D}_i - \mathbf{D}^* \rangle.
\end{align*}
Due to the strong convexity of $g_i$, we compute the mean of $\langle \nabla g_i(\mathbf{D}_i), \mathbf{D}_i - \mathbf{D}^* \rangle$ over $(\mathbf{z}_i, \mathbf{x}_i)$ so that
\begin{align*}
{\cal E}(\langle \nabla g_i(\mathbf{D}_i), \mathbf{D}_i - \mathbf{D}^* \rangle)  = {\cal E}( \langle \nabla g_i(\mathbf{D}_i) - \nabla g_i(\mathbf{D}^*), \mathbf{D}_{i}-\mathbf{D}^*\rangle)  \ge
\frac{\beta}{2} {\cal E}( \| \mathbf{D}_i - \mathbf{D}^* \|^2).
\end{align*}
Combining the above inequalities, we have
\begin{align*}
{\cal E}(\| \mathbf{D}_{i+1} - \mathbf{D}\|^2) &\leq  {\cal E}(\| \mathbf{D}_i - \mathbf{D} ^*\|^2) + \eta_i^2 C^2 -  \eta_i\beta{\cal E}( \|\mathbf{D}_i - \mathbf{D}^*\|^2)\\
&\leq (1-\beta \eta_i) {\cal E}(\| \mathbf{D}_i - \mathbf{D}^*\|^2) + \eta_i^2 C^2.
\end{align*}
By induction, it follows that
\begin{equation*}
{\cal E}(\| \mathbf{D}_{i+1} -\mathbf{D}\|^2)\le \prod_{j=1}^i (1-\beta\eta_j) {\cal E}(\|\mathbf{D}_1- \mathbf{D}^*\|^2) + \sum_{j=1}^i \prod_{k=j+1}^i (1-\beta\eta_k) C^2 \eta_j^2.
\end{equation*}
Thus, we have
\[
{\cal E}(\| \mathbf{D}_{i+1} - \mathbf{D}^* \|^2 ) \leq  \frac{1}{i+1} {\cal E}(\|\mathbf{D}_1- \mathbf{D}^*\|^2) +  \frac{C^2}{\beta^2}\frac{\ln(i+1)}{i+1},
\]
where we have used $\displaystyle \sum_{j=1}^{i+1}\frac{1}{j} > \ln (i+1) + O(1/i+1)$~(\cite{boyd2004convex}).
\end{proof}

\begin{Prop}\label{prop:lai}
Let $a_k, k\ge 1$ be a positive sequence. If $a_k, k\ge 1$ satisfy the following
\small
\begin{equation}
\label{eq:ak}
 a_{k+1}\le a_k + \frac{1}{k^{1+\epsilon}}, \quad \forall k\ge 1,
\end{equation}
\normalsize
then the sequence $a_k, k\ge 1$ converges.
\end{Prop}

\emph{Proof.}
For convenience, let $\epsilon=1/2$. Because $k \ge 1$ in the assumption, so that we can have $\sqrt{k(k+1)}(\sqrt{k}+\sqrt{k+1}) \ge \sqrt{kk} (\sqrt{k}+\sqrt{k})=2k\sqrt{k}$. Then when $\epsilon=1/2$, we can rewrite Eq.~\ref{eq:ak} to $a_{k+1}\le a_k + \frac{1}{k^{1+\frac{1}{2}}} = a_k + \frac{1}{k\sqrt{k}}, \quad \forall k\ge 1.$

It follows that
\begin{align*}
a_{k+1}\le a_k + \frac{1}{k\sqrt{k}} &\le a_k + \frac{2}{\sqrt{k(k+1)}(\sqrt{k}+\sqrt{k+1})} = a_k+ \frac{2}{\sqrt{k}}- \frac{2}{\sqrt{k+1}}.
\end{align*}
\normalsize
Let $b_n= a_n+ \dfrac{2}{\sqrt{k}}$. Thus, $0\le b_{k+1}\le b_k$ and hence, $b_k, k\ge 1$ are convergent. Let us say $b_k\to a^*$, that is, $a_k+ \dfrac{2}{\sqrt{k}}\to a^*$. Similarly, we can verify that it is true for any $\epsilon>0$. Therefore, it follows that $a_k\to a^*$.  \hfill $\square$

Now we are ready to give the main result of the SCC convergence analysis.
\begin{Them}
Suppose $\mathbf{D}^*\in \mathbb{C}$ is a local minimizer such that the mean value ${E}(\nabla g_i(\mathbf{D}^*))=0$ over random variables $(\mathbf{z}_i, \mathbf{x}_i)$ according to Proposition~\ref{claim:sgd-dec} and Proposition~\ref{prop:di-d*} such that
\begin{align*}
M_k= &\frac{1}{n}\sum_{i=1}^n ( \langle( \mathbf{D}^*\mathbf{z}_i^{k-1} -x_i)\mathbf{z}_i^{k-1}, (\mathbf{D}_{i}^k- \mathbf{D}^*)\rangle +
\frac{1}{2}\|\mathbf{z}_i^{k-1}\|^2\|(\mathbf{D}^k_{i}-\mathbf{D}^*)\|^2 \\
-&(\langle (\mathbf{D}^*\mathbf{z}_i^k - x_i)\mathbf{z}_i^k, (\mathbf{D}_{i+1}^k- \mathbf{D}^*)\rangle +
\frac{1}{2}  \|\mathbf{z}_i^k\|^2\|\mathbf{D}^k_{i+1}-\mathbf{D}^*\|^2 )) = O(1/k^{1+\epsilon}),
\end{align*}
as $k\to \infty$ for a positive $\epsilon>0$. Due to Proposition~\ref{prop:di-d*}, we know that $\mathbf{D}^k_i \to \mathbf{D}^*$ in the following fashion as $\mathbf{D}_i - \mathbf{D}^* =O(\frac{1}{i}), \hbox{ as } i\to \infty.$ Then our algorithm converges.

\end{Them}
\emph{Proof.}
It is worth noting the $M_k$ can be rewrite into 

\begin{align*}
M_k= &\frac{1}{n}\sum_{i=1}^n ( \lang \nabla g_{i}(\mathbf{D}^*), \mathbf{D}_{i}^k- \mathbf{D}^*\rangle + \frac{1}{2}\|(\mathbf{D}^k_{i}-\mathbf{D}^*)\mathbf{z}_i^{k-1}\|^2 \\
-&(\langle\nabla g_{i+1}(\mathbf{D}^*), \mathbf{D}_{i+1}^k- \mathbf{D}^*\rangle +
\frac{1}{2}\|(\mathbf{D}^k_{i+1}-\mathbf{D}^*)\mathbf{z}_i^k\|^2 )).
\end{align*}

We have the Taylor expansion of $\sum f_i(\mathbf{D}^k_{i+1}, \mathbf{z}_i^k)$ at $D^*$ as follows:
\small
\begin{align*}
& \frac{1}{n}\sum_{i=1}^n  f_i(\mathbf{D}^*, \mathbf{z}_i^k) + \frac{1}{n}\sum_{i=1}^n (\langle \nabla g_{i+1}(\mathbf{D}^*), \mathbf{D}_{i+1}^k- \mathbf{D}^*\rangle + \frac{1}{2} \|(\mathbf{D}^k_{i+1}-\mathbf{D}^*)\mathbf{z}_i^k\|^2 ).
\end{align*}
\normalsize
Similar for $\sum f_i(\mathbf{D}^k_i, \mathbf{z}_i^{k-1})$, we also have Taylor expansion
\small
\begin{align*}
&\frac{1}{n}\sum_{i=1}^n  f_i(\mathbf{D}^*, \mathbf{z}_i^{k-1}) +\frac{1}{n}\sum_{i=1}^n (\langle \nabla g_{i}(\mathbf{D}^*), \mathbf{D}_{i}^k- \mathbf{D}^*\rangle + \frac{1}{2} \|(\mathbf{D}^k_{i}-\mathbf{D}^*)\mathbf{z}_i^{k-1}\|^2).
\end{align*}
\normalsize

Therefore, we mainly use Proposition~\ref{prop:exp-dic-dec} for the following proof. For each epoch $k$,
\small
\begin{align*}
\frac{1}{n} \sum_{i=1}^n f_i(\mathbf{D}^k_{i+1}, \mathbf{z}_i^k)  \leq  \frac{1}{n} \sum_{i=1}^n f_i(\mathbf{D}^k_i, \mathbf{z}_i^{k-1}).
\end{align*}
\normalsize
When $k$ goes infinity, we can rewrite $\mathbf{D}_i^k = \mathbf{D}_{(k-1)*n+i+1}=\mathbf{D}^*+ O(\frac{1}{kn})$ as $k\to \infty$. 
Thus, we have
\small
$$
\frac{1}{n}\sum_{i=1}^n f_i(\mathbf{D}^*, \mathbf{z}_i^k) \le   \frac{1}{n}\sum_{i=1}^n f_i(\mathbf{D}^*, \mathbf{z}_i^{k-1}) + M_k,
$$
\normalsize
where $M_k$ is the one as in the assumption of this theorem.
Given $M_k = O(1/{k^{1+\epsilon}})$ as $k\to \infty$ for $\epsilon>0$ and Proposition~\ref{prop:lai}, the new sequence $\dfrac{1}{n}\sum_{i=1}^n f_i(\mathbf{D}^*, \mathbf{z}_i^k) $ converges to limit ${\cal F}(\mathbf{D}^*, \mathbf{z}_1^*, \cdots, \mathbf{z}_n^*)$, where $\mathbf{z}_i^*$ is the limit of a sub-sequence of $\mathbf{z}_i^k$ for $i=1, \cdots, n$ as $\mathbf{z}_i^k, k\ge 1$ are bounded by Proposition~\ref{bound}.

Therefore, from the above discussion, 
$\frac{1}{n}\sum_{i=1}^n f_i(\mathbf{D}_{i+1}^k, \mathbf{z}_i^k) - \frac{1}{n}\sum_{i=1}^n f_i(\mathbf{D}^*, \mathbf{z}_i^{k}) \to 0$ and when $k\to \infty$, we conclude that $\lim_{k\to \infty} \frac{1}{n}\sum_{i=1}^n  f_i (\mathbf{D}^k_{i+1}, \mathbf{z}_i^{k}) = {\cal F}(\mathbf{D}^*, \mathbf{z}_i^*, \cdots, \mathbf{z}_n^*)$ so that our algorithm converges.  \hfill $\square$

\label{App:convergence}
